# Supplementary material for: Like Article, Like Audience: Enforcing Multimodal Correlations for Disinformation Detection
Source: arXiv:2108.13892 source file (2021-08-31)
Supplement: Supplementary file 1 [file appendix.tex]

\begin{table*}[]
    \centering
    \begin{tabular}{c|ccc|ccc|ccc|c}
        \toprule
        & \multicolumn{3}{c}{Politifact} & \multicolumn{3}{c}{Gossipcop} & \multicolumn{3}{c}{ReCOVery} & Reasoning \\ 
        \midrule
        & P & R & F1 & P & R & F1 & P & R & F1\\
        \midrule
        %$\lambda_1$=0, $\lambda_2$=0 & .74 & .68 & .66 & .85 & .85 & .84 & .84 & .84 & .83 \\
        %\midrule
        %$\lambda_1$=0.25, $\lambda_2$=0.25 & .74 & .68 & .66 & .85 & .85 & .84 & .82 & .83 & .81 \\
        %$\lambda_1$=0.25, $\lambda_2$=0.5 & .74 & .68 & .66 & .85 & .85 & .84 & .82 & .82 & .80 \\
        %\textbf{$\lambda_1$=0.25, $\lambda_2$=0.75} & \textbf{.74} & \textbf{.68} & \textbf{.66} & \textbf{.85} & \textbf{.85} & \textbf{.84} & \textbf{.84} & \textbf{.84} & \textbf{.83} \\
        %\midrule
        %$\lambda_1$=0.5, $\lambda_2$=0.25 & .71 & .65 & .61 & .84 & .84 & .82 & .79 & .79 & .75 \\
        %$\lambda_1$=0.5, $\lambda_2$=0.5 & .72 & .67 & .64 & .85 & .85 & .83 & .82 & .82 & .79 \\
        %$\lambda_1$=0.5, $\lambda_2$=0.75 & .74 & .68 & .66 & .85 & .85 & .83 & .82 & .82 & .79 \\
        %\midrule
        %$\lambda_1$=0.75, $\lambda_2$=0.25 & .76 & .57 & .44 & .81 & .80 & .77 & .80 & .73 & .62 \\
        %$\lambda_1$=0.75, $\lambda_2$=0.5 & .28 & .53 & .37 & .81 & .80 & .76 & .80 & .73 & .62 \\
        %$\lambda_1$=0.75, $\lambda_2$=0.75 & .28 & .53 & .37 & .82 & .81 & .78 & .80 & .73 & .62 \\
        %\midrule
        %$\lambda_1$=1, $\lambda_2$=1 & .28 & .53 & .37 & .55 & .75 & .64 & .53 & .73 & .61 \\
        %\midrule
        $\lambda_1$=1, $\lambda_2$=0, $\lambda_3$=0 & .74 & .68 & .66 & .85 & .85 & .84 & .84 & .84 & .83 & Only prediction loss \\
        \midrule
        $\lambda_1$=0.33, $\lambda_2$=0.33, $\lambda_3$=0.33 & .28 & .53 & .37 & .56 & .75 & .64 & .53 & .73 & .61 & All losses are equally important \\
        \midrule
        $\lambda_1$=0.5, $\lambda_2$=0.25, $\lambda_3$=0.25 & .79 & .65 & .59 & .84 & .84 & .82 & .79 & .78 & .72 & Distance losses are equally important, \\
        $\lambda_1$=0.8, $\lambda_2$=0.1, $\lambda_3$=0.1 & .74 & .68 & .66 & .85 & .85 & .84 & .83 & .83 & .81 & but prediction loss is most important \\
        \midrule
        $\lambda_1$=0.5, $\lambda_2$=0.5, $\lambda_3$=0 & .28 & .53 & .37 & .56 & .75 & .64 & .53 & .73 & .61 & Don't take into account user-user correlations\\
        $\lambda_1$=0.5, $\lambda_2$=0, $\lambda_3$=0.5 & .73 & .67 & .63 & .85 & .85 & .84 & .87 & .87 & .86 & Don't take into account article-user correlations\\
        \midrule
        $\lambda_1$=0.6, $\lambda_2$=0.1, $\lambda_3$=0.3 & .74 & .68 & .66 & .85 & .85 & .84 & .83 & .83 & .81 & Prediction > user-user > article-user loss \\
        $\lambda_1$=0.6, $\lambda_2$=0.3, $\lambda_3$=0.1 & .75 & .67 & .62 & .85 & .85 & .83 & .82 & .80 & .76 & Prediction > article-user > user-user loss \\
        \bottomrule
    \end{tabular}
    \caption{Experiments with various $\lambda$-values for $CNN_{+user/d}$.}
    \label{tab:my_label}
\end{table*}

\begin{table*}[]
    \centering
    \begin{tabular}{c|ccc|ccc|ccc|c}
        \toprule
        & \multicolumn{3}{c}{Politifact} & \multicolumn{3}{c}{Gossipcop} & \multicolumn{3}{c}{ReCOVery} & Reasoning \\ 
        \midrule
        & P & R & F1 & P & R & F1 & P & R & F1\\
        \midrule
        $\lambda_1$=1, $\lambda_2$=0, $\lambda_3$=0 & .67 & .67 & .66 & .83 & .84 & .83 & .85 & .85 & .84 & Only prediction loss \\
        \midrule
        $\lambda_1$=0.33, $\lambda_2$=0.33, $\lambda_3$=0.33 & .72 & .70 & .69 & .85 & .85 & .85 & .87 & .88 & .87 & All loss functions are equally important \\
        \midrule
        $\lambda_1$=0.5, $\lambda_2$=0.25, $\lambda_3$=0.25 & .73 & .72 & .71 & .84 & .85 & .84 & .87 & .88 & .87 & Distance losses are equally important, \\
        $\lambda_1$=0.8, $\lambda_2$=0.1, $\lambda_3$=0.1 & .70 & .70 & .69 & .84 & .84 & .84 & .85 & .85 & .84 & but prediction loss is most important \\
        \midrule
        $\lambda_1$=0.5, $\lambda_2$=0.5, $\lambda_3$=0 & .71 & .70 & .69 & .85 & .85 & .85 & .88 & .88 & .88 & Don't take into account user-user correlations\\
        $\lambda_1$=0.5, $\lambda_2$=0, $\lambda_3$=0.5 & .70 & .68 & .67 & .84 & .84 & .84 & .84 & .84 & .83 & Don't take into account article-user correlations\\
        \midrule
        $\lambda_1$=0.6, $\lambda_2$=0.1, $\lambda_3$=0.3 & .70 & .70 & .69 & .84 & .85 & .84 & .86 & .86 & .85 & Prediction > user-user > article-user loss\\
        $\lambda_1$=0.6, $\lambda_2$=0.3, $\lambda_3$=0.1 & .74 & .73 & .73 & .84 & .85 & .84 & .86 & .86 & .85 & Prediction > article-user > user-user loss \\
        \bottomrule
    \end{tabular}
    \caption{Experiments with various $\lambda$-values for $HAN_{+user/d}$.}
    \label{tab:my_label}
\end{table*}
